# Supplementary material for: HiFiHR: Enhancing 3D Hand Reconstruction from a Single Image via High-Fidelity Texture
Source: arXiv:2308.13628 ancillary file (2023-08-25)
Supplement: Supplementary file 1 [file HiFiHR_suppl.pdf]

# HiFiHR: Enhancing 3D Hand Reconstruction from a Single Image via High-Fidelity Texture

## Supplementary Material

Jiayin Zhu, Zhuoran Zhao, Linlin Yang, and Angela Yao

National University of Singapore
{zhujiayin,zhuoran.zhao}@u.nus.edu, {yangll,ayao}@comp.nus.edu.sg

## 1 Loss function formulas

### 1.1 Geometry loss

The full set of geometry loss contains a joint location loss, a vertex location loss, a bone direction loss, and an edge length loss. We introduce the formulas for each loss term under different levels of supervision.

In the **fully supervised setting**, the joint location loss $\mathcal{L}_{jnt}$ encourages estimated 3D keypoints $J_i'$ to be close to their corresponding ground truth $J_i$, where $i \in [1, N]$ and $N$ is the sample number in the training set. We also include the vertex location loss $\mathcal{L}_{vert}$ to shorten the distance between estimated 3D vertices $V_i'$ and their corresponding ground truth $V_i$. Following the dataset setting, there are 21 keypoints and 778 vertices for each hand sample. The formulas are:

$$\mathcal{L}_{jnt} = \frac{1}{k} \sum_{n=1}^{k} \mathrm{L1}(J_{i,n}, J'_{i,n}), \tag{1}$$

$$\mathcal{L}_{vert} = \frac{1}{v} \sum_{m=1}^{v} \mathrm{L1}(V_{i,m}, V'_{i,m}), \tag{2}$$

where $k = 21, v = 778$, and we use L1 loss to calculate the distance between each location pair. The bone direction loss $\mathcal{L}_{direc}$ forces the bone alignment between estimation and ground truth, where each bone is the vector between two adjacent keypoints:

$$\mathcal{L}_{direc} = \frac{1}{k-1} \sum_{n=2}^{k} \|(J_{i,n} - J_{i,n-1}) - (J'_{i,n} - J'_{i,n-1})\|_2^2. \tag{3}$$

Lastly, the edge length loss $\mathcal{L}_{len}$ acts to encourage the length of estimated mesh edges to be close to the ground truth:

$$\mathcal{L}_{len} = \frac{1}{v-1} \sum_{m=2}^{v} \|(V_{i,m} - V_{i,m-1}) - (V'_{i,m} - V'_{i,m-1})\|_2^2. \tag{4}$$

In the **weakly supervised setting**, only the 2D joint location loss $\mathcal{L}_{jnt}^{2D}$ and the 2D bone direction loss $\mathcal{L}_{direc}^{2D}$ are included. Compared with $\mathcal{L}_{jnt}$ which is in 3D space, $\mathcal{L}_{jnt}^{2D}$ is computed between the 2D ground truth keypoints $J_i^{2D} \in \mathbb{R}^2$ and the projected $J_i'$:

$$\mathcal{L}_{jnt}^{2D} = \frac{1}{k}\sum_{n=1}^{k} L1(J_{i,n}^{2D}, \text{proj}(J'_{i,n})), \tag{5}$$

where proj$(\cdot)$ denotes the projection function from 3D to 2D space, and proj$(J_i') \in \mathbb{R}^2$. Similarly, $\mathcal{L}_{direc}^{2D}$ is also computed in 2D space:

$$\mathcal{L}_{direc}^{2D} = \frac{1}{k-1}\sum_{n=2}^{k} \|(J_{i,n}^{2D} - J_{i,n-1}^{2D}) - (\text{proj}(J'_{i,n}) - \text{proj}(J'_{i,n-1}))\|_2^2. \tag{6}$$

Moreover, in the **self-supervised setting**, we utilize the 2D joint location loss $\mathcal{L}_{jnt\_con}^{2D}$ and the 2D bone direction loss $\mathcal{L}_{direc\_con}^{2D}$ with detected noisy 2D joints $J_i^{det}$, conditioned by the confidence scores, $con_i$ and $con_i^{bone}$, provided by OpenPose [1]:

$$\mathcal{L}_{jnt\_con}^{2D} = \frac{1}{k}\sum_{n=1}^{k} con_{i,n} \cdot L1(J_{i,n}^{det}, \text{proj}(J'_{i,n})), \tag{7}$$

$$\mathcal{L}_{direc\_con}^{2D} = \frac{1}{k-1}\sum_{n=2}^{k} con_{i,n}^{bone} \cdot \|(J_{i,n}^{det} - J_{i,n-1}^{det}) - (\text{proj}(J'_{i,n}) - \text{proj}(J'_{i,n-1}))\|_2^2. \tag{8}$$

### 1.2 Texture reconstruction consistency

The texture reconstruction consistency $\mathcal{L}_{tex}$ consists of a pixel loss, a mean color loss, a silhouette loss, an SSIM loss, and a perceptual loss. The pixel loss $\mathcal{L}_{pix}$ forces each foreground pixel in the rendered image $I_i'$ to be close to the pixel at the same location in the original image $I_i$, and the mean color loss $\mathcal{L}_{color}$ encourages the foreground RGB color to be similar:

$$\mathcal{L}_{pix} = \mathbb{E}[\text{L1}(I_i \odot M_i, I_i' \odot M_i)], \tag{9}$$

$$\mathcal{L}_{color} = \text{L1}(\mathbb{E}[I_i \odot M_i], \mathbb{E}[I_i' \odot M_i]), \tag{10}$$

where $\odot$ denotes element-wise multiplication, and $\mathbb{E}[\cdot]$ denotes the expectation. The silhouette loss $\mathcal{L}_{sil}$ calculate the pixel level L1 loss between the rendered mask $M_i'$ and its corresponding ground truth $M_i$:

$$\mathcal{L}_{sil} = \mathbb{E}[\text{L1}(M_i, M_i')]. \tag{11}$$

The SSIM loss $\mathcal{L}_{ssim}$ is calculated using the structural similarity between the two images [3], and the perceptual loss $\mathcal{L}_{perc}$ calculates the difference between deep features of two images extracted by a pretrained AlexNet network [2]:

$$\mathcal{L}_{ssim} = 1 - \text{SSIM}(I_i \odot M_i, I_i' \odot M_i), \tag{12}$$

$$\mathcal{L}_{perc} = \|\text{LPIPS}(I_i \odot M_i) - \text{LPIPS}(I'_i \odot M_i)\|_2^2. \tag{13}$$

Note that in the self-supervised settings, because the ground truth mask is not accessible, we use the rendered mask $M'_i$ to replace $M_i$ in $\mathcal{L}_{ssim}$ and $\mathcal{L}_{perc}$.

## 2 Effect of each loss function

We conduct more ablation studies on losses to verify the effect of each loss function. Experiments are conducted on the FreiHAND test set [4]. Tab. 1 shows the results, where we divide the experiments into three groups, *i.e.*, geometry-related loss, texture-related loss, and regularization. The full 3D geometry loss ($\mathcal{L}_{geo}^{3D}$) provides the strongest supervision with the best result, which is our baseline. In each following experiment, we change one specific component. Replacing the 3D geometry loss with 2D ($\mathcal{L}_{geo}^{2D}$) and noisy geometry loss ($\mathcal{L}_{geo}^{2D\_det}$) leads to worse performance. Removing $\mathcal{L}_{direc}$ results in a noticeable increase of 0.05 in both MPJPE and MPVPE, demonstrating the importance of $\mathcal{L}_{direc}$. Removing $\mathcal{L}_{len}$ leads to a slight increase in MPJPE and a marginal increase in MPVPE, which proves that $\mathcal{L}_{len}$ is helpful for mesh prediction.

In terms of texture reconstruction consistency loss, removing $\mathcal{L}_{low-level}$ contributes to the best MPJPE, MPVPE, suggesting that $\mathcal{L}_{low-level}$ introduces noise to fully-supervised pose and shape estimation. However, we note that although removing $\mathcal{L}_{low-level}$ results in the highest PSNR, the generated hand texture lacks realism from the human perspective (see Fig. 3). Hence, we believe that $\mathcal{L}_{low-level}$ remains crucial, and the current metrics for evaluating texture quality may have limitations. On the other hand, removing $\mathcal{L}_{high-level}$ results in a slight increase in MPJPE, MPVPE and a decrease in PSNR, suggesting $\mathcal{L}_{high-level}$ is important for learning high-fidelity texture. Fig. 3 presents the visualization of different combinations of texture-related losses, showing our full loss $\mathcal{L}_{tex}$ provides the best texture result.

$\mathcal{L}_{regu}$ provides regularizations on hand parameters and are crucial for network convergence. Removing $\mathcal{L}_{regu}$ results in performance degradation.

**Table 1.** Ablation study on losses.

| Methods | Description | MPJPE↓ | MPVPE↓ | PSNR↑ |
|---|---|---|---|---|
| $\mathcal{L}_{geo}^{3D}$ | Full supervision, baseline | 1.21 | 1.23 | 19.547 |
| $\mathcal{L}_{geo}^{2D}$ | Weak supervision | 1.23 | 1.24 | 20.008 |
| $\mathcal{L}_{geo}^{2D\_det}$ | Self supervision | 1.31 | 1.33 | 20.036 |
| w/o $\mathcal{L}_{geo}$ | Self* supervision | 1.66 | 1.65 | 17.876 |
| w/o $\mathcal{L}_{direc}$ | w/o bone direction loss | 1.26 | 1.28 | 19.490 |
| w/o $\mathcal{L}_{len}$ | w/o edge length loss | 1.23 | 1.27 | 19.146 |
| w/o $\mathcal{L}_{low-level}$ | w/o low-level texture loss | 1.19 | 1.21 | 19.880 |
| w/o $\mathcal{L}_{high-level}$ | w/o high-level texture loss | 1.23 | 1.25 | 19.051 |
| w/o $\mathcal{L}_{tex}$ | w/o texture reconstruction consistency | 1.21 | 1.24 | - |
| w/o $\mathcal{L}_{regu}$ | w/o regularization | 1.47 | 1.51 | 18.988 |

## 3 More qualitative results

We show additional qualitative results of our method in Figs. 1 and 2.

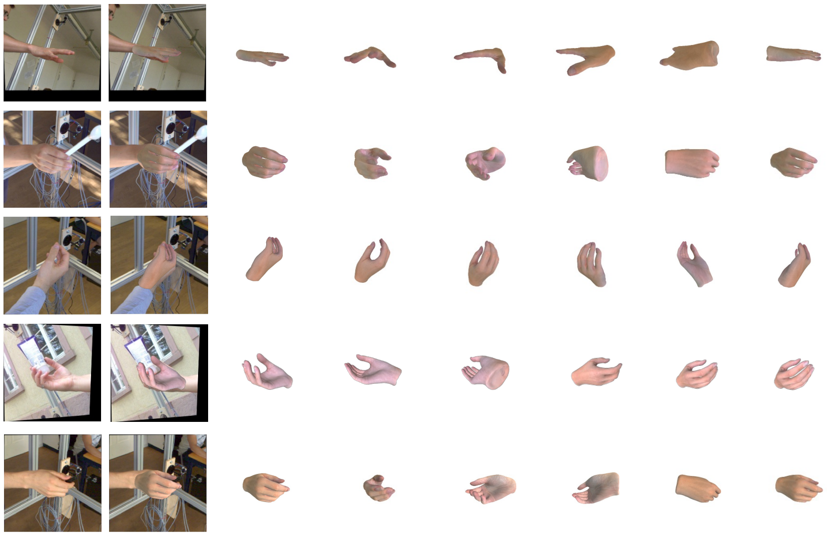

**Fig. 1.** Additional qualitative results on the FreiHAND testing set. From left to right: input image, reconstructed 3D hand mesh (projected to image), 3D hand mesh from various views.

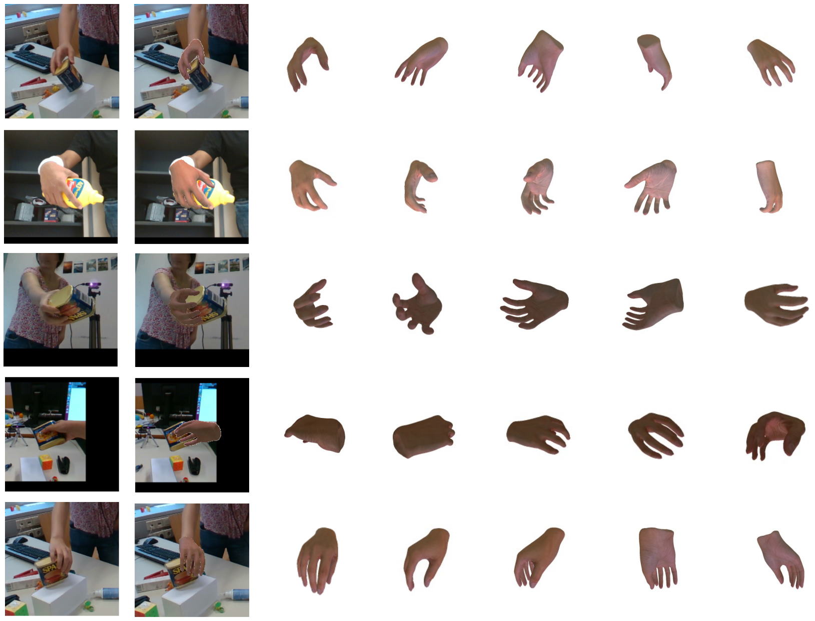

**Fig. 2.** Additional qualitative results on the HO-3Dv2 testing set. From left to right: input image, reconstructed 3D hand mesh (projected to image), 3D hand mesh from various views.

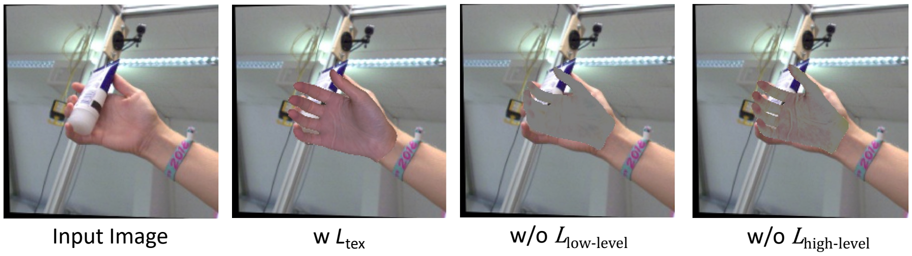


**Fig. 3.** Reconstructed 3D hand mesh trained with $\mathcal{L}_{tex}$, without $\mathcal{L}_{low-level}$ and without $\mathcal{L}_{high-level}$. Our full setting $\mathcal{L}_{tex}$ provides the best texture result.

## References

1. Cao, Z., Simon, T., Wei, S.E., Sheikh, Y.: Realtime multi-person 2d pose estimation using part affinity fields. In: Computer Vision and Pattern Recognition. pp. 7291–7299 (2017)
2. Krizhevsky, A., Sutskever, I., Hinton, G.E.: Imagenet classification with deep convolutional neural networks. Communications of the ACM **60**(6), 84–90 (2017)
3. Wang, Z., Bovik, A., Sheikh, H., Simoncelli, E.: Image quality assessment: from error visibility to structural similarity. IEEE Transactions on Image Processing **13**(4), 600–612 (2004)
4. Zimmermann, C., Ceylan, D., Yang, J., Russell, B., Argus, M., Brox, T.: Freihand: A dataset for markerless capture of hand pose and shape from single rgb images. In: International Conference on Computer Vision. pp. 813–822 (2019)
